# Supplementary material for: Real-space observation of emergent complexity of phase evolution in micrometer-sized IrTe$_2$ crystals
Source: arXiv:2110.05813 source file (2021-10-12)
Supplement: Supplementary file 1 [file Oike_Supplementary_211012.pdf]

Supplemental Material for

# Real-space observation of emergent complexity of phase evolution in micrometer-sized $IrTe_2$ crystals

H. Oike[1,2†], K. Takeda[1], M. Kamitani[2], Y. Tokura[1,2,3] and F. Kagawa[1,2†]

[1] *Department of Applied Physics and Quantum-Phase Electronics Centre (QPEC), The University of Tokyo, Tokyo 113-8656, Japan*

[2] *RIKEN Center for Emergent Matter Science (CEMS), Wako 351-0198, Japan*

[3] *Tokyo College, University of Tokyo, Tokyo 113-8656, Japan*

† To whom correspondence should be addressed. E-mail: oike@ap.t.u-tokyo.ac.jp; kagawa@ap.t.u-tokyo.ac.jp

## Sample preparation

Bulk single crystals of $IrTe_2$ were synthesized using the Te-flux method according to the literature [S1]. Submicrometer-thick thin plates were exfoliated from the same bulk crystal with Scotch tape and transferred onto a silicon (Si) substrate. The sample thickness and volume of each thin plate were derived from the topography, which was measured using closed-loop atomic force microscopy (AFM). Scanning Raman microscopy was performed mainly for samples #1 (perimeter $l \approx 77$ μm, thickness $d \approx 480$ nm, and volume $V \approx 160$ μm$^3$) and #2 ($l \approx 49$ μm, $d \approx 160$ nm, and $V \approx 22$ μm$^3$).

In the even smaller sample #5 (perimeter $l \approx 28$ μm, thickness $d \approx 110$ nm, and volume $V \approx 6$ μm$^3$), the D-to-UD transition temperature was appreciably lower than that in the bulk sample (Fig. S4), implying that another mechanism begins to play a role in the emergent phase-change properties. This observation is consistent with a recent experimental study, which reports that the D-to-UD transition temperature decreases when the thickness is below 150 nm [S2]. In the present study, we excluded such a small sample to highlight the complexity of the phase evolution caused by sample miniaturization while minimizing other effects, such as enhanced surface contributions to the total free energy.

For atomically thin films, it is known that a substrate can exert an appreciable local strain [S3, S4]. We thus checked whether some inhomogeneity is present in our thin-flake samples by using scanning Raman microscopy and found that the Raman spectrum at each pixel exhibited no appreciable spatial dependence (Fig. S2). Thus, within experimental resolution, our thin-flake samples, in which the thickness is 160 nm or greater, appear to be homogeneous, thereby indicating that there are no inhomogeneous strains from the substrate with a detectable magnitude (in terms of scanning Raman microscopy).

## Scanning Raman microscopy

The excitation laser was a frequency-doubled Nd:YAG diode-pumped solid-state laser (wavelength: 532 nm). The laser intensity during image scans was 5 mW; this did not cause considerable sample heating near room temperature, as the observed transition temperatures from the Ir-dimerized (D) phase to the Ir-undimerized (UD) phase upon heating were nearly the same as those in resistivity measurements. For detection, we used a single-mode optical fiber and a charge-coupled spectrometer with a grating of 1,800 lines mm$^{-1}$. All measurements were performed with linear laser polarization. To clarify the probing depth of the present experiment, we measured how the signal intensity of the Si substrate underneath the $IrTe_2$ thin flakes varied with flake thickness (Fig. S1). From this result, the probing depth was estimated to be ≈ 10 nm.

## Data processing of the raw Raman spectra

The typical pixel size of the domain images in the present study is ~400×400 nm$^2$, and a Raman spectrum, $f(\boldsymbol{r}, \omega)$, was acquired at each pixel centered at $\boldsymbol{r}$, where $\boldsymbol{r} = (x, y)$ and $\omega$ represent the two-dimensional coordinates of a position and the Raman shift, respectively. We often found that spike signals mixed into the Raman spectrum, which were probably due to cosmic rays; we therefore removed the spike signals before performing the detailed analysis. Our system was equipped with two longpass filters (532 US LPF, Iridian Spectral Technologies and LP03-532RE-25, Semrock) so that the Raman scattering light below 60 cm$^{-1}$ was cut off

before entering the spectrometer. Nevertheless, a finite signal level far below the cutoff wavenumber remained, which could reasonably be attributed to the system background. Specifically, a nearly flat residual signal level between –100 $cm^{-1}$ and –300 $cm^{-1}$ was subtracted from the obtained Raman spectrum as the system background.

## Estimation of the volume fractions of the two competing phases

To extract the volume fraction of the D phase at each pixel (in particular, pixels close to the UD/D phase boundaries), we should consider the fact that the spectrum intensity at each pixel depends on the amount of scattering light collected by the objective lens and is thus affected by geometrical factors, such as (i) the surface roughness and (ii) the drift of the distance between the sample surface and the objective lens during scanning (typically, the drift is ~100 nm). Thus, the Raman spectrum at an arbitrary position in the sample can be represented as

$$f(\boldsymbol{r},\omega) = A(\boldsymbol{r})\left[\phi_{\mathrm{UD}}(\boldsymbol{r})\bar{f}_{\mathrm{UD}}(\omega) + \phi_{\mathrm{D}}(\boldsymbol{r})\bar{f}_{\mathrm{D}}(\omega)\right],$$

where $A(\boldsymbol{r})$ represents a scale factor caused by the geometrical factors; $\phi_{\mathrm{UD}}(\boldsymbol{r})$ and $\phi_{\mathrm{D}}(\boldsymbol{r})$ [$\phi_{\mathrm{UD}}(\boldsymbol{r}) + \phi_{\mathrm{D}}(\boldsymbol{r}) \equiv 1$] are the volume fractions of the UD and D phases at a given pixel, respectively; and $\bar{f}_{\mathrm{UD}}(\omega)$ and $\bar{f}_{\mathrm{D}}(\omega)$ are the spectra of the UD and D phases, respectively, for which the intensity is well averaged by collecting a large amount of data. All the Raman spectra were successfully fitted with this equation, and thus, two-dimensional $\phi_{\mathrm{UD}}(\boldsymbol{r})$ maps were constructed, as shown in Figs. 1−4 in the main text. Most areas of the sample corresponded to either $\phi_{\mathrm{UD}}(\boldsymbol{r}) \approx 1$ (the UD phase) or $\phi_{\mathrm{D}}(\boldsymbol{r}) \approx 1$ (the D phase), but at pixels on or near the UD/D domain boundaries, these values appreciably deviated from 1. The macroscopic volume fraction of the D phase, $\phi_{\mathrm{D}}$, was thus obtained by

$$\phi_{\mathrm{D}} = \frac{\int_S \, dxdy \, \phi_{\mathrm{D}}(x,y)}{\int_S \, dxdy},$$

where $S$ denotes the entire area of the thin plate.

## Correction of the image distortion

A piezo element inherently exhibits nonlinear and hysteretic deformation in response to an applied external voltage. As our scanning Raman system is a so-called open-loop system, the positional information of the piezo elements is not directly monitored, and the voltage applied to the piezo elements is not feedbacked. Consequently, the scanned Raman images inevitably include extrinsic distortion originating from the piezo elements. By contrast, in a so-called closed-loop system, the positional information is always monitored, and the applied voltage is feedbacked; thus, such an extrinsic distortion is already minimized in the scanned image. As an example, a domain image scanned with an open-loop system and a topographic image scanned with a closed-loop system are displayed in Figs. S7(a) and S7(b), respectively. The outer shape of the specimen shown in Fig. S7(a) is slightly different from that in Fig. S7(b) because Fig. S7(a) includes the image distortions.

To remove false distortions, we performed a post-image processing step with the ImageJ Fiji program (https://imagej.net/Fiji/Downloads). We used the topographic AFM image obtained with a closed-loop system [Fig. S7(b)] as the undistorted reference image. In the image-conversion process, we referred to the outer shape of the specimen and the positions of the bumps and dips on the surface; then, the distorted domain images [Fig. S7(a)] were corrected so that these two-dimensional topographic aspects agreed with those in the reference image [Fig. S7(b)]. Thus, the distortion-corrected domain image was obtained as shown in Fig. S7(c).

## Resistivity measurements

The resistivity of the thin plates was measured with a conventional four-probe method. Gold electrodes were fabricated with photolithography, and the electrodes on the sample surface were connected with those on the substrate by tungsten deposition using a focused-ion beam. An a.c. voltage excitation was generated by a lock-in amplifier (Signal Recovery, 7270) and applied to the sample. Signals from the voltage probes were amplified with a low-noise

preamplifier (NF Corporation, SA-410F3 or Stanford Research, SR560) and measured with the lock-in amplifier.

## Supplementary reference


[S1] M. J. Eom, K. Kim, Y. J. Jo, J. J. Yang, E. S. Choi, B. I. Min, J.-H. Park, S.-W. Cheong, and J. S. Kim, Phys. Rev. Lett. **113**, 266406 (2014).

[S2] S. Park, S. Y. Kim, H. K. Kim, M. J. Kim, T. Kim, H. Kim, G. S. Choi, C. J. Won, S. Kim, K. Kim, E. F. Talantsev, K. Watanabe, T. Taniguchi, S-W. Cheong, B. J. Kim, H. W. Yeom, J. Kim, T-H. Kim, and J. S. Kim, Nat. Commun. **12**, 3157 (2021).

[S3] C. Neumann, S. Reichardt, P. Venezuela, M. Drögeler, L. Banszerus, M. Schmitz, K. Watanabe, T. Taniguchi, F. Mauri, B. Beschoten, S.V. Rotkin and C. Stampfer, Nat. Commun. **6**, 8429 (2015).

[S4] N. Poccia, S. Y. F. Zhao, H. Yoo, X. Huang, H. Yan, Y. S. Chu, R. Zhong, G. Gu, C. Mazzoli, K. Watanabe, T. Taniguchi, G. Campi, V. M. Vinokur, and P. Kim, Phys. Rev. Mat. **4**, 114007 (2020).

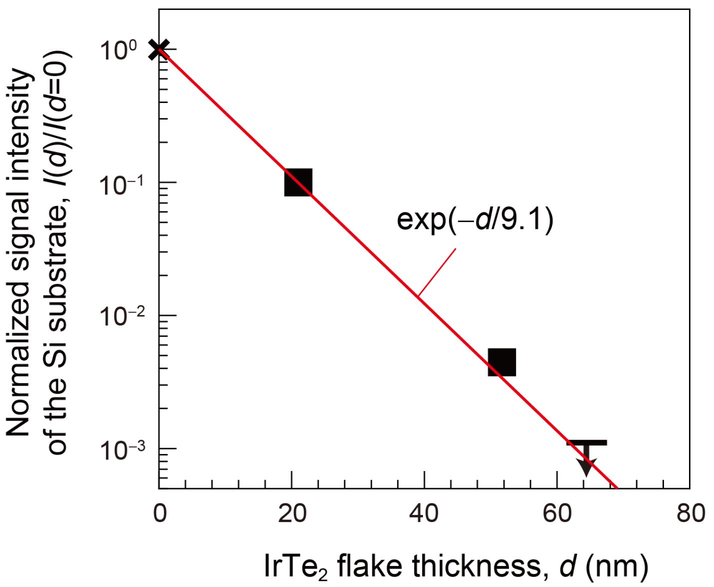


Fig. S1: Normalized signal intensity of the Si substrate underneath the $IrTe_2$ thin flakes as a function of the thickness of the flake. The result is fitted with $I(d)/I(d=0) = \exp(-d/\lambda)$, where $I$, $d$, and $\lambda$ represent the signal intensity, flake thickness, and probing depth. Thus, $\lambda \approx$ 10 nm is obtained.

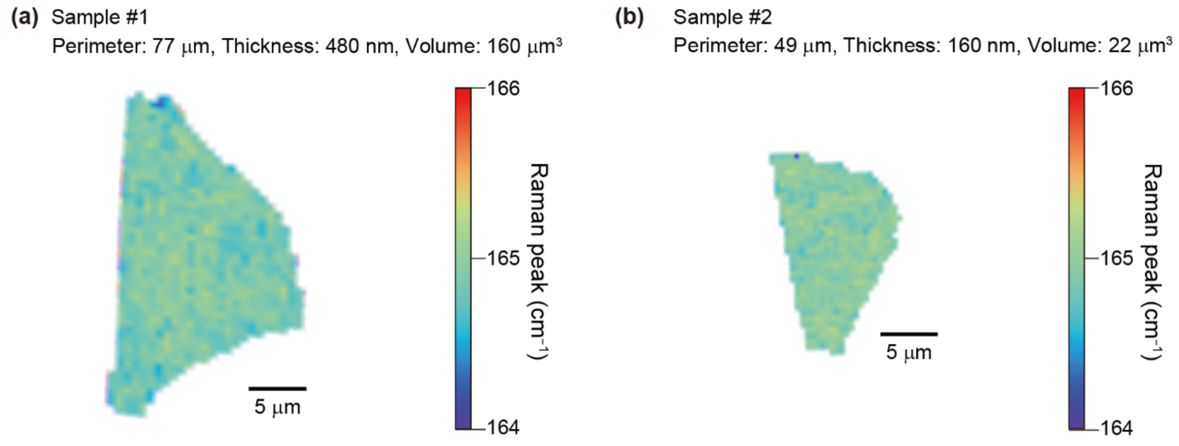


Fig. S2: Spatial dependence of the Raman peak around ~165 $cm^{-1}$ in samples #1 (a) and #2 (b). The measurements were done for the fully UD phase at 280 K. No spatially correlated fluctuations were found, thereby indicating that the thin flakes appeared to be homogeneous with respect to scanning Raman microscopy.

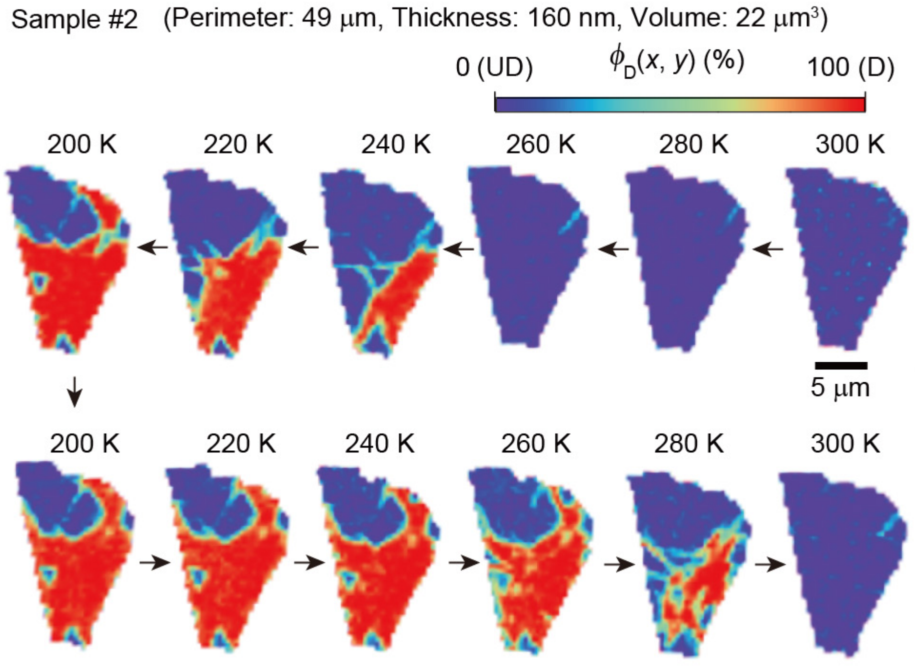


Fig. S3: Consecutive domain images of sample #2 during a thermal cycle of 300 → 200 → 300 K. From these images, the temperature evolution of the Ir-dimerized (D) phase was obtained, as shown in Fig. 2(b) in the main text.

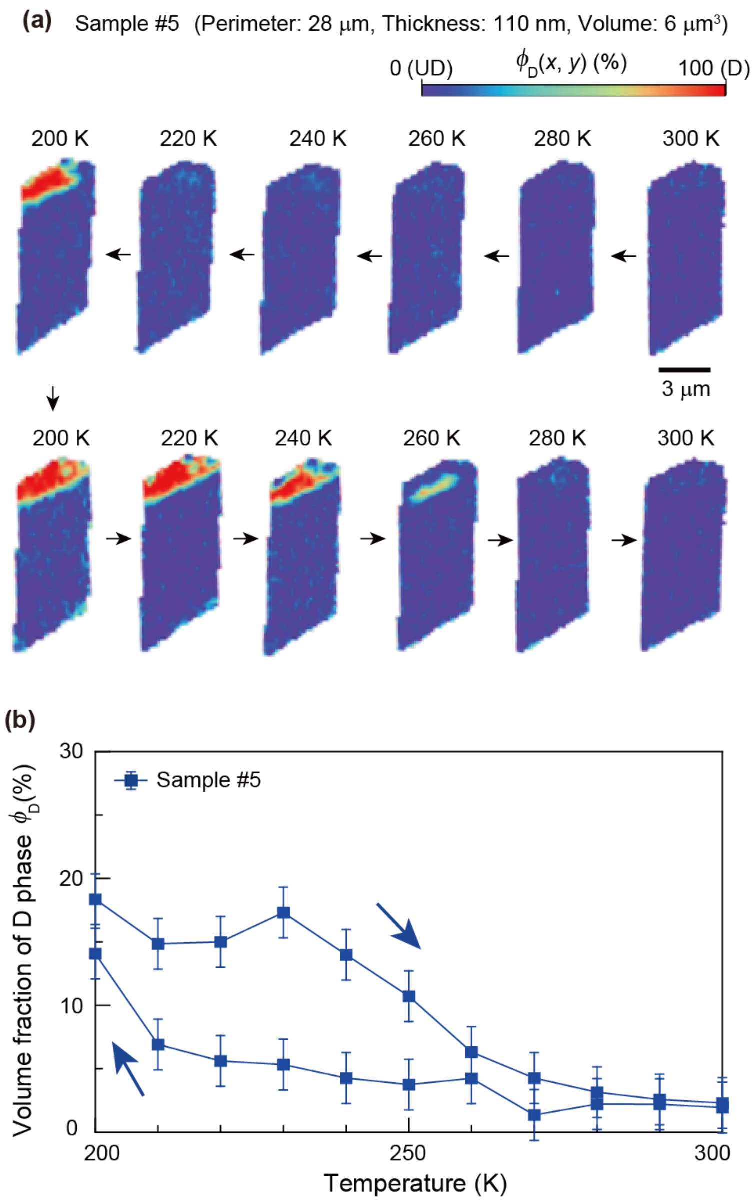


Fig. S4: Temperature evolution of the Ir-dimerized (D) domain in sample #5 during a thermal cycle. (a) Consecutive domain images for a thermal cycle of 300 → 200 → 300 K. (b) Temperature evolution of the volume fraction of the D phase in sample #5. The perimeter, thickness and volume of sample #5 are 28 μm, 110 nm and 6 $\mu m^3$, respectively.

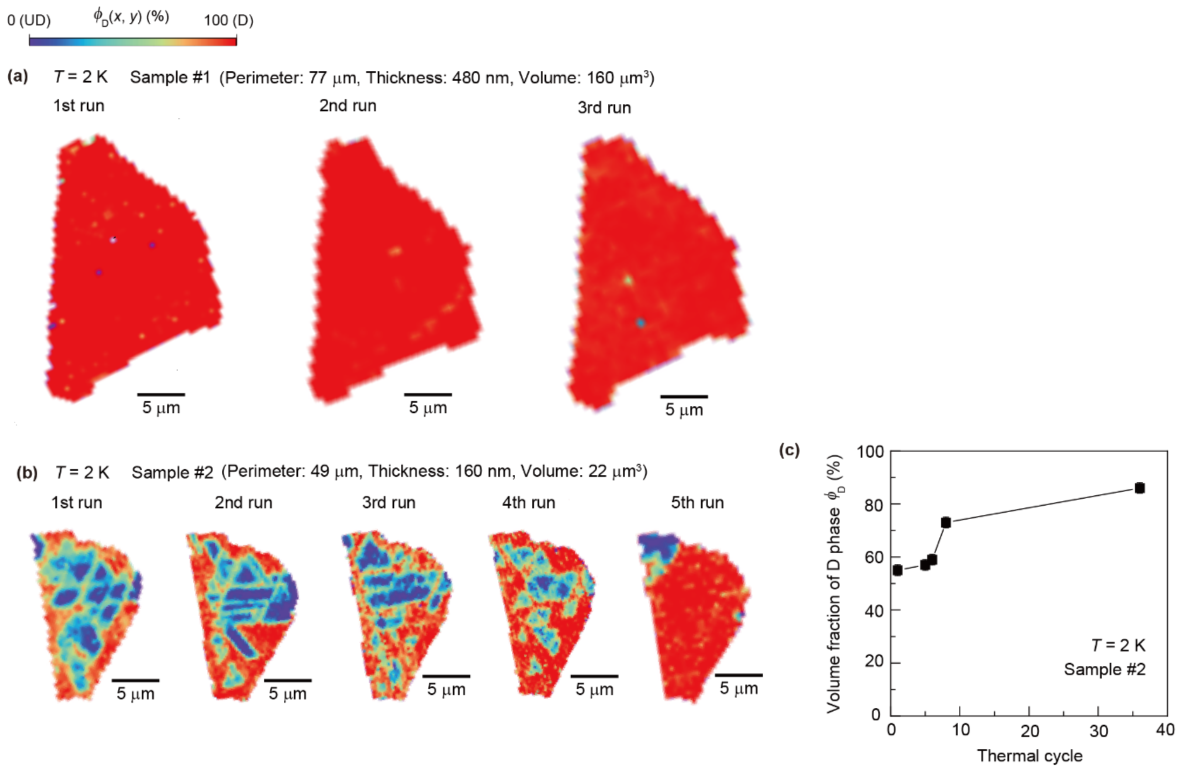


Fig. S5: Repeated domain imaging at the lowest temperature, measured for samples #1 (a) and #2 (b). In every sequence, the sample was cooled from 300 K (fully Ir-undimerized state) to 2 K without laser irradiation. (c) Volume fraction of the D phase at the lowest temperature in sample #2, plotted against the number of phase transitions experienced. Sample #2, it was cooled to 2 K five times, but in reality, there were more temperature cycles that did not reach 2 K. We counted the number of times that the specimen underwent the structural phase transition, and the volume fraction at the lowest temperature was plotted against this number. We found that as the thermal cycle was repeated, the volume fraction of the D phase at the lowest temperature tended to increase. This tendency suggests that new nucleation centers are yielded by the repeated structural phase transition, although the experimental resolution does not allow us to identify them directly.

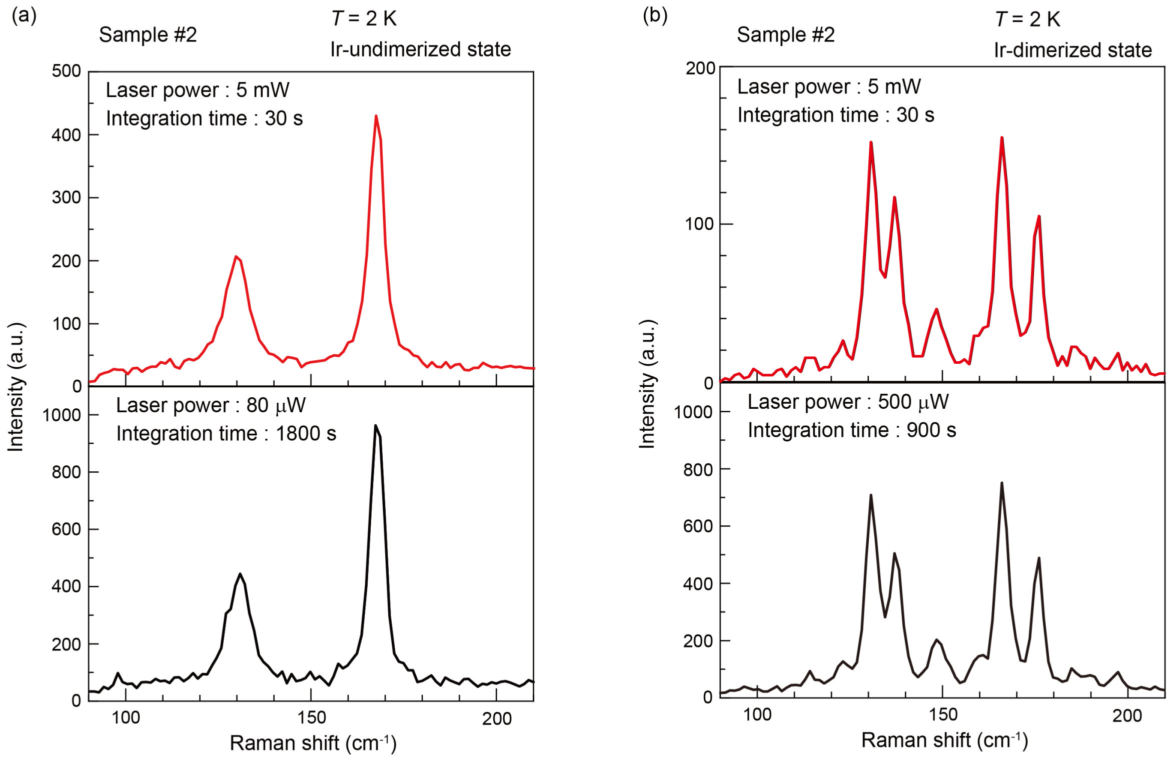


Fig. S6: Excitation power dependence of the Raman spectra of the Ir-undimerized phase (a) and the Ir-dimerized phase (b) at the lowest temperature. The measurement was performed at a pixel in the Ir-undimerized domain or a pixel in the Ir-dimerized domain of the phase mixture [Fig. 4(c) in the main text].

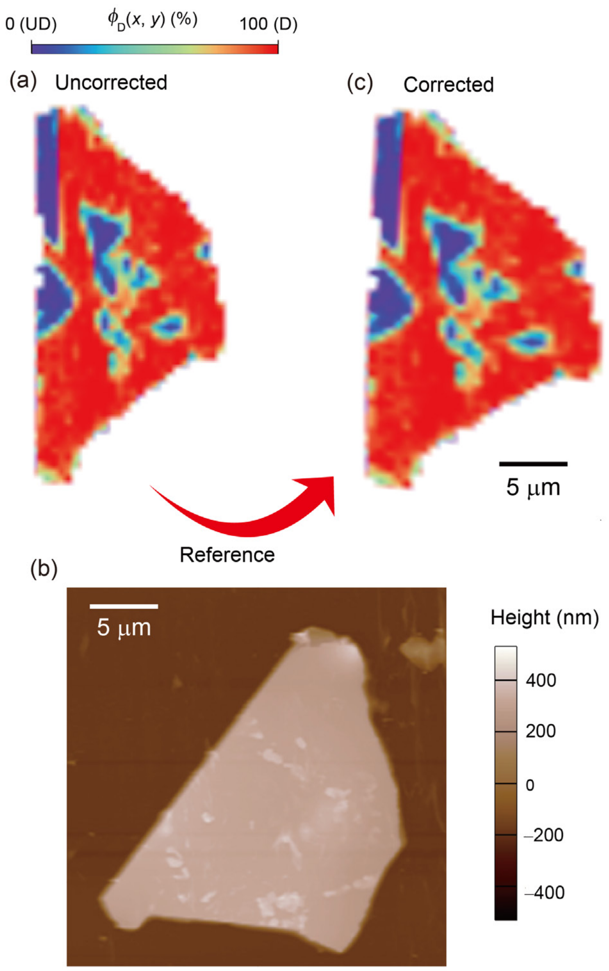


Fig. S7: Correction of the image distortion caused by scanning with the open-loop system. (a) Distorted domain image obtained with the open-loop system. (b) Topographic atomic force microscopy (AFM) image obtained with a closed-loop system. The false distortion due to the piezo elements is thought to be minimized in this image, which can therefore be used as a reference in distortion correction. (c) Distortion-corrected domain image.
